# Supplementary material for: Making Large Language Models Better Planners with Reasoning-Decision Alignment
Source: arXiv:2408.13890 source file (2024-08-25)
Supplement: Supplementary file 1 [file X_suppl.tex]

% \clearpage
% \setcounter{page}{1}

% \begin{table*}[t]
%        \centering
%        \setlength\tabcolsep{4.3pt}
%        \begin{tabularx}{0.81\textwidth}{c|ccc|c|ccc|c}
%        \toprule
%        \multirow{2}{*}{Training samples} &\multicolumn{4}{c|}{L2 (m) $\downarrow$} & \multicolumn{4}{c}{Collision (\%) $\downarrow$} \\
%        \cmidrule(){2-9}
%        & 1s & 2s & 3s & Avg. & 1s & 2s & 3s & Avg. \\
%        \toprule
%        10$\%$ & 0.29 & 1.44 & 2.98 & 1.57 & 0.03 & 0.48 & 2.08 & 0.86 \\
%        50$\%$ & 0.25 & 0.79 & 1.66 & 0.89 & 0.00 & 0.18 & 1.18 & 0.45 \\
%     \rowcolor{mygray}   100$\%$ & 0.23 & 0.73 & 1.54 & \textbf{0.80} & 0.00 & 0.13 & 0.83 & \textbf{0.32} \\
%        \bottomrule
%        \end{tabularx}
%    \caption{Few-shot learning. With a small number of samples, \name{} performs competitive results.}
%    \label{tab:ablation_few_shot}
% \end{table*}
% \maketitlesupplementary

\section{Additional Details}
\subsection{Implementation Details}
We adapt LLaVa\cite{liu2023llava} as the foundation LLM in our \name{}.
To denote the final trajectory output format, we add special tokens "<SOT>" (Start of Trajectory) and "<EOT>" (End of Trajectory) at the beginning and end of the trajectory, respectively.
In the perception data annotated by DriveLM\cite{sima2023drivelm}, it is necessary to predict the specific coordinates of each object in the image. 
However, due to the difficulty and lower priority of the coordinate prediction task, and to encourage the model to focus more on overall logical reasoning rather than excessively focusing on detailed predictions, we remove the coordinate part during the training process, retaining only the object's camera position in the image, \ie, {\textsf{<c4, CAM\_FRONT>}}.
Finally, we train \name{} for 10 epochs with LoRA\cite{hu2021lora} fine-tuning strategy.

\section{Additional Results}
\subsection{Few-shot learning}
To assess the model's ability in logical reasoning and causal inference, we conducte few-shot experiments using 10$\%$, 50$\%$, and 100$\%$ of the training data, as shown in \ref{tab:ablation_few_shot}. 
Even with a small number of samples, \ie, 10$\%$ of the training data, \name{} demonstrate a competitive end-to-end decision-making capability, despite the full dataset containing only 4072 samples. 
As the amount of data increases, the model consistently achieves better performance.

% \subsection{Computational Complexity}

\section{Additional Visualizations}
\subsection{More Qualitative Results}
As illustrated in \cref{fig:visualization}, we presents additional examples showcasing the logical reasoning of \name{}.
By responding to COT prompts related to perception, prediction, and behavior, \name{} can consistently reason across various scenarios such as straight driving and turning, ultimately predicting accurate driving trajectory.

% \vspace{-10mm}
\subsection{Video Demo}
In addition to the figures, we have attached a video demo in the supplementary materials, which consists of hundreds of frames that provide a more comprehensive evaluation of our proposed approach.
% We have attached a video demo in the supplementary materials.

\begin{figure*}[htp]
  \centering
    % \fbox{\rule{0pt}{2in} \rule{.9\linewidth}{0pt}}
    % \vspace{-7mm}
    \includegraphics[width=1\linewidth]{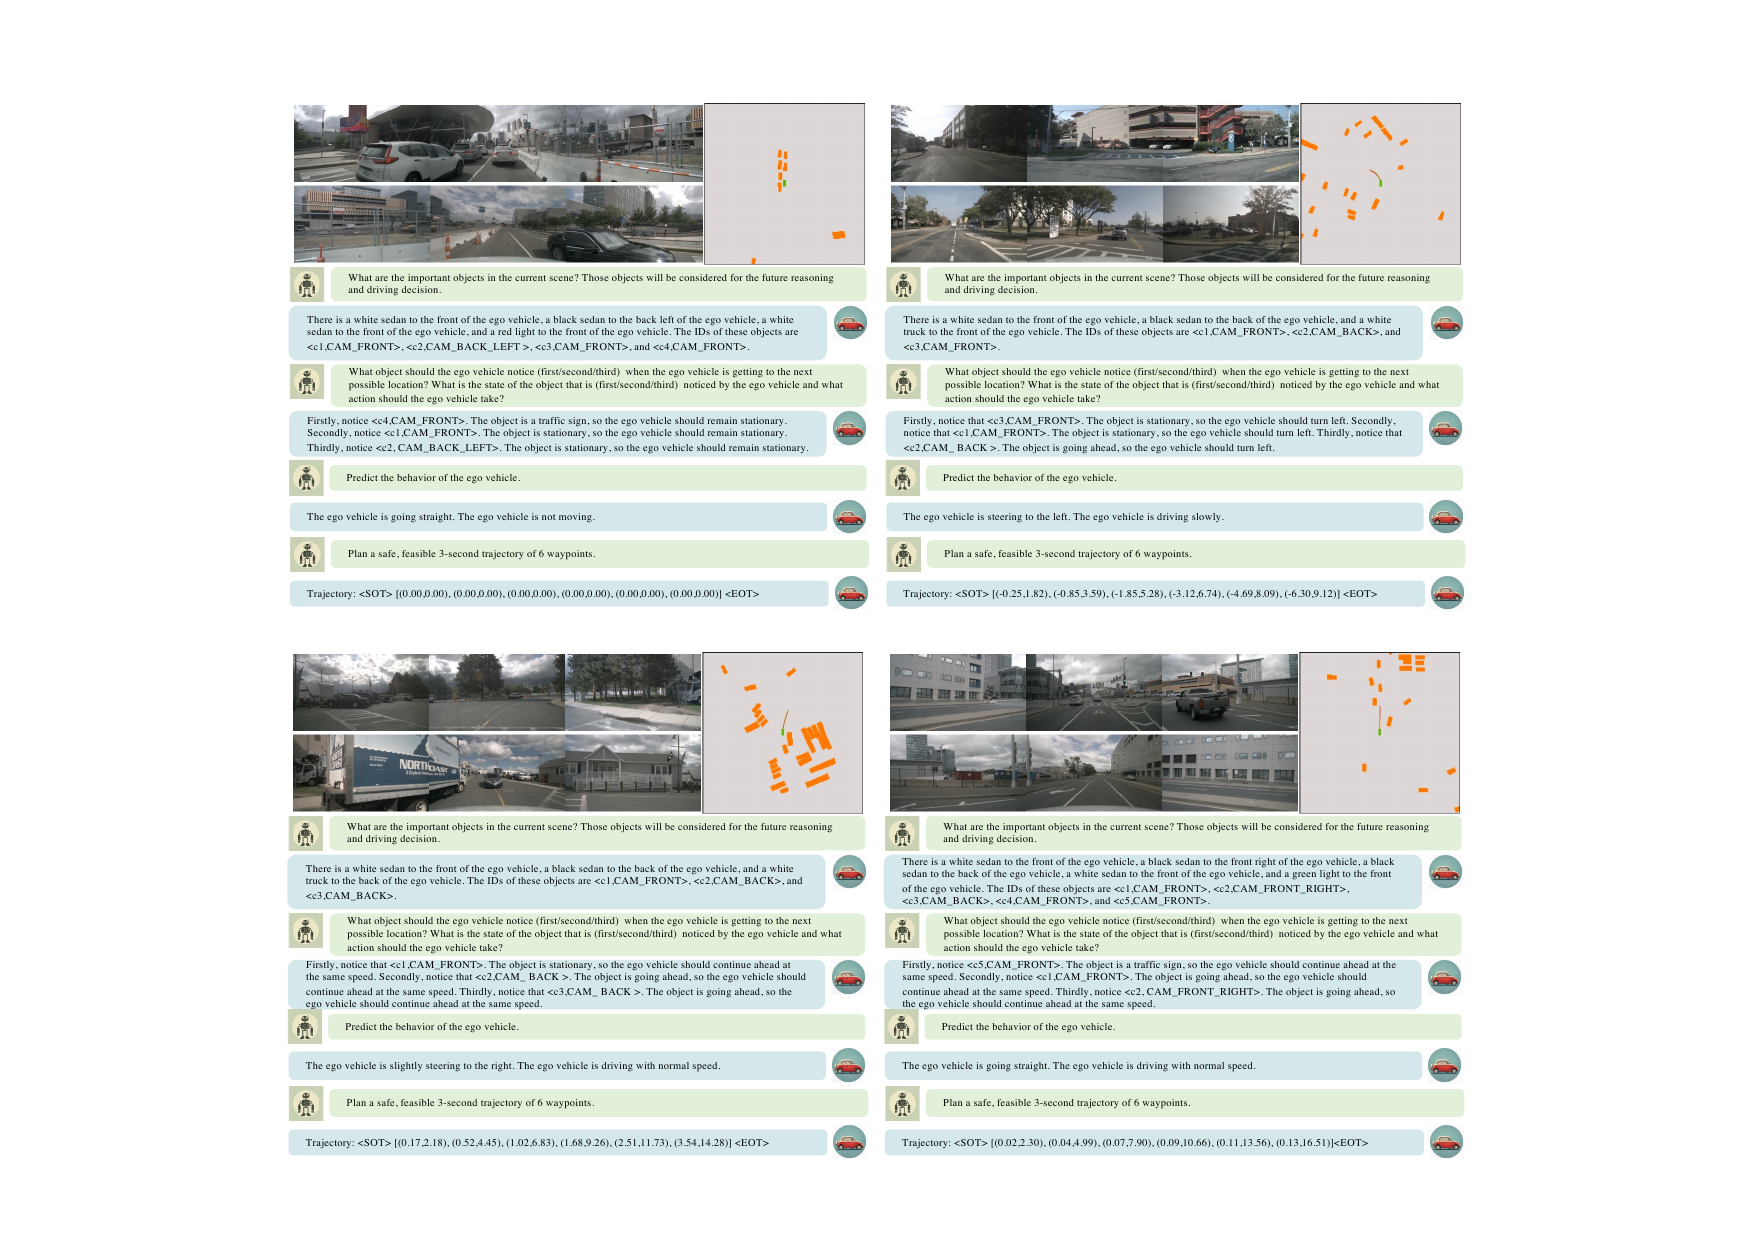}
  % \caption{\textbf{Framework of \name{}. Generally, \name{} takes as input the multi-view images, ego status and CoT prompt. We propose\xd{detailed caption}}}
  \caption{Examples of the logical reasoning and trajectory planning of \name{}. The planned trajectory and gt trajectory are in green and red respectively.}
  \label{fig:visualization}
  % \vspace{-10mm}
\end{figure*}

% \section{Appendix}
% \label{sec:rationale}
% %
% Having the supplementary compiled together with the main paper means that:
% %
% \begin{itemize}
%     \item The supplementary can back-reference sections of the main paper, for example, we can refer to \cref{sec:intro};
%     \item The main paper can forward reference sub-sections within the supplementary explicitly (e.g. referring to a particular experiment);
%     \item When submitted to arXiv, the supplementary will already included at the end of the paper.
% \end{itemize}
% %
% To split the supplementary pages from the main paper, you can use \href{https://support.apple.com/en-ca/guide/preview/prvw11793/mac#:~:text=Delete%20a%20page%20from%20a,or%20choose%20Edit%20%3E%20Delete).}{Preview (on macOS)}, \href{https://www.adobe.com/acrobat/how-to/delete-pages-from-pdf.html#:~:text=Choose%20%E2%80%9CTools%E2%80%9D%20%3E%20%E2%80%9COrganize,or%20pages%20from%20the%20file.}{Adobe Acrobat} (on all OSs), as well as \href{https://superuser.com/questions/517986/is-it-possible-to-delete-some-pages-of-a-pdf-document}{command line tools}.
