# Supplementary material for: Making Large Language Models Better Planners with Reasoning-Decision Alignment
Source: arXiv:2408.13890 source file (2024-08-25)
Supplement: Supplementary file 2 [file suppl.tex]

% \begin{table*}[t]
%        \centering
%        \setlength\tabcolsep{4.3pt}
%        \begin{tabularx}{0.81\textwidth}{c|ccc|c|ccc|c}
%        \toprule
%        \multirow{2}{*}{Training samples} &\multicolumn{4}{c|}{L2 (m) $\downarrow$} & \multicolumn{4}{c}{Collision (\%) $\downarrow$} \\
%        \cmidrule(){2-9}
%        & 1s & 2s & 3s & Avg. & 1s & 2s & 3s & Avg. \\
%        \toprule
%        10$\%$ & 0.29 & 1.44 & 2.98 & 1.57 & 0.03 & 0.48 & 2.08 & 0.86 \\
%        50$\%$ & 0.25 & 0.79 & 1.66 & 0.89 & 0.00 & 0.18 & 1.18 & 0.45 \\
%     \rowcolor{mygray}   100$\%$ & 0.23 & 0.73 & 1.54 & \textbf{0.80} & 0.00 & 0.13 & 0.83 & \textbf{0.32} \\
%        \bottomrule
%        \end{tabularx}
%    \caption{Few-shot learning. With a small number of samples, \name{} performs competitive results.}
%    \label{tab:ablation_few_shot}
% \end{table*}
